# Supplementary material for: ViLBERT: Pretraining Task-Agnostic Visiolinguistic Representations for Vision-and-Language Tasks
Source: arXiv:1908.02265 source file (2019-08-06)
Supplement: Supplementary file 1 [file supplement.tex]

\documentclass{article}

% if you need to pass options to natbib, use, e.g.:
%    \PassOptionsToPackage{sort&compress}{natbib}
% before loading neurips_2019

% ready for submission
% \usepackage{neurips_2019}

% to compile a preprint version, e.g., for submission to arXiv, add add the
% [preprint] option:
%     \usepackage[preprint]{neurips_2019}

% to compile a camera-ready version, add the [final] option, e.g.:
\usepackage[nonatbib]{style/neurips_2019}

%stuff to hack the bib into sorting citation by order of ¥ and grouping citiations
\usepackage[sort&compress]{natbib}
\setcitestyle{numbers}
\citestyle{plain}
\bibliographystyle{unsrtnat}

\usepackage[utf8]{inputenc} % allow utf-8 input
\usepackage[T1]{fontenc}    % use 8-bit T1 fonts
\usepackage{hyperref}       % hyperlinks
\usepackage{url}            % simple URL typesetting
\usepackage{booktabs}       % professional-quality tables
\usepackage{multirow}
\usepackage{amsfonts}       % blackboard math symbols
\usepackage{nicefrac}       % compact symbols for 1/2, etc.
\usepackage{microtype}      % microtypography
\usepackage{epigraph}
\usepackage{soul}
\usepackage[dvipsnames]{xcolor}
\usepackage{paralist}
\usepackage{graphicx}
\usepackage{subcaption}

\input{style/macros.tex}
\input{style/space_saver.tex}
\usepackage{style/mysymbols}

%\title{Multi-modal Bert: Towards a Universal Grounding Machine for Vision-And-Language Tasks}
%\title{VL-Bert: Towards Universal Grounded Representations for Vision-and-Language Tasks}
%\title{\vlbert: Learning Task-Agnostic Joint Representations for Vision and Language}
%\title{\vlbert: Task-Agnostic\\ Vision-and-Language Pretraining}
\title{Supplemental for \vlbert: Pretraining Task-Agnostic Models for Vision-and-Language Problems}

% The \author macro works with any number of authors. There are two commands
% used to separate the names and addresses of multiple authors: \And and \AND.
%
% Using \And between authors leaves it to LaTeX to determine where to break the
% lines. Using \AND forces a line break at that point. So, if LaTeX puts 3 of 4
% authors names on the first line, and the last on the second line, try using
% \AND instead of \And before the third author name.

\author{%
  David S.~Hippocampus\thanks{Use footnote for providing further information
    about author (webpage, alternative address)---\emph{not} for acknowledging
    funding agencies.} \\
  Department of Computer Science\\
  Cranberry-Lemon University\\
  Pittsburgh, PA 15213 \\
  \texttt{hippo@cs.cranberry-lemon.edu} \\
  % examples of more authors
  % \And
  % Coauthor \\
  % Affiliation \\
  % Address \\
  % \texttt{email} \\
  % \AND
  % Coauthor \\
  % Affiliation \\
  % Address \\
  % \texttt{email} \\
  % \And
  % Coauthor \\
  % Affiliation \\
  % Address \\
  % \texttt{email} \\
  % \And
  % Coauthor \\
  % Affiliation \\
  % Address \\
  % \texttt{email} \\
}

\begin{document}

\maketitle

temp

\bibliography{bib/main.bib}

\end{document}
